# Supplementary material for: A General Framework for Multi-fidelity Bayesian Optimization with Gaussian Processes
Source: arXiv:1811.00755 source file (2018-11-02)
Supplement: Supplementary file 1 [file appendix-proof-expexp.tex]

\begin{algorithm}[t!]
  \nl {\bf Input}: {Budget $\budget$; cost $\costof{i}$ for all fidelities $i \in [\targetfid]$}; joint GP prior on $\{\fidelity_i, \noise_i\}_{i\in[\targetfid]}$\\ % between $\fidelity_i$ and noise $$. \\
  \Begin{
    % \nl $\alpha = \frac{\max_\ex \infgain{\action{\ex, \targetfid}}}{\sqrt{\budget} \costof{\targetfid}} $ \\
    \nl $\selected \leftarrow \emptyset$ \\
    \nl $B \leftarrow \budget$ \tcc*{initialize remainig budget}
    \tcc{explore with low fidelity}
    \nl $\epselected \leftarrow$ \explorelf $\paren{B, [\costof{\fid}], \GP{\{\utility_\fid, \noise_\fid\}_{\fid\in[\targetfid]}}, \selected}$ \\
    \While{$B > 0$} % outer loop
    {
      \tcc{select target fidelity}
      \nl $\ex^* \leftarrow \sfgpopt(\GP{\{\tarf, \noise_\targetfid\}}, \bobs_{\selected \cup \epselected})$ \label{alg:expexp:ln:sfgpopt}\\
      \nl $\selected \leftarrow \selected \cup \epselected \cup \{\action{\ex^*,\targetfid}\}$\\
      \nl $B \leftarrow \budget - \Cost_\selected$ \tcc*{update remaining budget}
    }
    \nl {\bf Output}: Optimizer of the target function $\tarf$ \\
  }
  \caption{\algExploreExploit}\label{alg:explore-then-exploit}
\end{algorithm}

Let us use $\costOfSet{\selected} := \sum_{\action{\ex, \fid} \in \selected} \costof{\fid} $ to denote the cost of the set of actions $\selected$. Further, let $\selectedTar$ be a set that only consists of actions from the target fidelity, i.e., $\forall \action{\ex, \fid} \in \selectedTar: \fid = \targetfid$, and $\epselected$ be the set of (low fidelity) actions selected by \explorelf. Define
\begin{align*}
  &\gamma \triangleq \max_{\selected: \costOfSet{\selected} \leq \budget}\infgain{\bobs_{\selected}} \\
  &\gamma_m \triangleq \max_{\selectedTar: \costOfSet{\selectedTar}\leq \budget}\infgain{\bobs_{\selectedTar}}\\
  &\gamma_L \triangleq \infgain{\bobs_{\eplow}}
\end{align*}
In words, $\gamma$ is the maximal mutual information one can gather about the payoff function $\tarf$
by performing actions at \emph{all fidelities} under budget $\budget$; $\gamma_m$ is the maximal information one can gather about $\tarf$ by performing actions at the \emph{target fidelity} under budget $\budget$, and $\gamma_L$ denotes the mutual information between $\tarf$ and
% the observations $\bobs_\eplow$ of
the low fidelity actions $\eplow$ selected by \algExploreExploit.

We first establish the regret bound of \algExploreExploit via the following lemma.
% following lemma, stating the regret of
\begin{lemma}\label{lem:explore-then-exploit}
  % Let $\budget$ be the budget. % and let $\gamma_m \triangleq \max_{\selected: \sum_{\action{\ex, \targetfid} \in \selected} \costof{\fid} \leq \Cost}\infgain{\bobs_{\selected}}$ be .
  Assume that with budget $\budget$, \sfgpopt has an expected cumulative regret at most $\sqrt{\constgeneral \budget \gamma_m}$, where $\constgeneral$ is some constant.
  \algExploreExploit (\algref{alg:explore-then-exploit}) achieves expected cumulative regret
  \begin{align}
    \cumreg(\policy,\budget) \leq \sqrt{\constgeneral \budget \paren{\gamma - \gamma_L}} + \gamma_L \cdot \littleO{\sqrt{\budget}}
  \end{align}
\end{lemma}
\begin{proof}
  \algExploreExploit starts by exploring $\tarf$ with low fidelity actions $\eplow $ selected by \explorelf (\algref{alg:explorelf}). According to the stopping condition of \algref{alg:explorelf} at Line \ref{alg:explorelf:ln:infgaincheck},
  we know that when \explorelf terminates, the selected low fidelity actions $\eplow$ satisfy
  \begin{align*}
    % &\frac{\infgain{\bobs_{\eplow \cup \{ \action{\ex^*, \fid^*} \} } }}{\paren{\Cost_\eplow + \costof{\fid^*}}} < \beta \\&
    \frac{\infgain{\bobs_{\eplow } }}{{\Cost_\eplow}} = \frac{\gamma_L}{\Cost_\eplow} \geq \beta.
  \end{align*}
  Recall that $\beta = \frac{1}{\littleO{\sqrt{\budget}}}$. We thus have
  \begin{align}
    \Cost_\eplow \leq \frac{\gamma_L}{\beta} = \gamma_L \cdot \littleO{\sqrt{\budget}}. \label{eq:expexp-cost-lf-ub}
  \end{align}
  % \begin{align*}
  %   \action{\ex^*, \fid^*} =
  %   \argmax_{\action{\ex, \fid}: \costof{\fid} \leq \budget-\Cost_\eplow - \costof{\targetfid}} \frac{\condinfgain{\obs_{\action{\ex, \fid}}}{\bobs_{\eplow}}}{\costof{\fid}}
  % \end{align*}
  % When \explorelf terminates, we have
  % \begin{align*}
  %   \frac{\infgain{\bobs_{\eplow \cup \{ \action{\ex^*, \fid^*} \} } }}{\paren{\Cost_\eplow + \costof{\fid^*}}} < \beta
  % \end{align*}
  % where
  % \begin{align*}
  %   \action{\ex^*, \fid^*} =
  %   \argmax_{\action{\ex, \fid}: \costof{\fid} \leq \budget-\Cost_\eplow - \costof{\targetfid}} \frac{\condinfgain{\obs_{\action{\ex, \fid}}}{\bobs_{\eplow}}}{\costof{\fid}}
  % \end{align*}

  After the first episode selected by \explorelf, % \algref{alg:explorelf},
  \algExploreExploit % (\algref{alg:explore-then-exploit})
  then continues with picking actions at the target fidelity $\targetfid$ using \sfgpopt (line \ref{alg:expexp:ln:sfgpopt} of \algref{alg:explore-then-exploit}). Because only the first episode of \algExploreExploit could contain any low fidelity actions, the number of episodes is
  \begin{align*}
    k = \frac{\budget - \epcost}{\costof{\targetfid}}
  \end{align*}

  By definition of the cumulative regret (Eq.~\eqref{eq:cumregret}), we get
  \begin{align}
    \cumreg(\policy,\budget)
    &= \frac{\budget}{\costof{\targetfid}} \tarf^* - \sum_{j=1}^k \reward(\eplowat{j} \cup \{\tarselectedat{j}\}) \nonumber \\
    &= \frac{\budget}{\costof{\targetfid}} \tarf^* - \paren{\reward(\eplowat{1} \cup \{\tarselectedat{j}\}) + \sum_{j=2}^k \reward(\cancelto{\emptyset}{\eplowat{j}} \cup \{\tarselectedat{j}\})} \nonumber \\
    &= \frac{\budget}{\costof{\targetfid}} \tarf^* - \paren{\cancelto{0}{\reward(\eplowat{1})} + \sum_{j=1}^k \reward\paren{\tarselectedat{j}}} \nonumber \\
    &= \frac{\budget}{\costof{\targetfid}} \tarf^* -  \sum_{j=1}^{k} \tarf\paren{\ex^{\paren{j}}} \nonumber \\
    &= \paren{\frac{\budget}{\costof{\targetfid}}-k} \tarf^* +  \sum_{j=1}^{k} \paren{\tarf^* - \tarf\paren{\ex^{\paren{j}}}} \nonumber \\
    &= {\frac{\epcost}{\costof{\targetfid}}} \tarf^* +  \sum_{j=1}^{k} \paren{\tarf^* - \tarf\paren{\ex^{\paren{j}}}} \label{eq:explore-then-exploit-regret-intermediate}
  \end{align}
  % \yuxin{Make sure here the notation of an episode is consistent with the definition: Episode $\eplow_j \cup \{\action{\ex_j, \targetfid}\}$}.
  % By Theorem 5 of \citet{srinivas10gaussian},
  Notice that the first term on the RHS of Eq.~\eqref{eq:explore-then-exploit-regret-intermediate} is bounded by
  \begin{align}
    \frac{\epcost}{\costof{\targetfid}} \tarf^* \stackrel{\eqref{eq:expexp-cost-lf-ub}}{\leq} \gamma_L \cdot \littleO{\sqrt{\budget}} \frac{\tarf^*}{\costof{\targetfid}} = \gamma_L \cdot \littleO{\sqrt{\budget}} \label{eq:expexp:lf-regret},
  \end{align}
  and the second term is the regret of \sfgpopt under budget $\budget-\epcost$. By the chain rule of mutual information,
  \begin{align*}
    \max_{\selectedTar: \costOfSet{\selectedTar}\leq \budget - \epcost}\condinfgain{\bobs_{\selectedTar}}{\bobs_\eplow}
    &\leq \max_{\selected: \costOfSet{\selected} \leq \budget}\infgain{\bobs_{\selected}} - \infgain{\bobs_{\eplow}} = \gamma - \gamma_L.
  \end{align*}
  We thus have
  \begin{align}
    \sum_{j=1}^{k} \paren{\tarf^* - \tarf(\ex_j)} \leq \sqrt{C \paren{\budget-\epcost} (\gamma - \gamma_L)} \leq \sqrt{C \budget (\gamma - \gamma_L)}. \label{eq:expexp:sf-regret}
  \end{align}
  Combining Eq.~\eqref{eq:expexp:lf-regret}, \eqref{eq:expexp:sf-regret} with Eq.~\eqref{eq:explore-then-exploit-regret-intermediate} completes the proof.
\end{proof}

% Our next lemma, \lemref{lem:exp-vs-sfgpout} states that the cumulative regret bound of \explorelf is at least at good as \sfgpopt.
% \begin{lemma}\label{lem:exp-vs-sfgpout}
%   Fix $\budget$. The expected cumulative regret of \algExploreExploit (\algref{alg:explore-then-exploit}) is no worse that the regret of \sfgpopt.
% \end{lemma}
% \begin{proof}
%   \yuxin{This is not true --- let's take a different approach. Let's not try to bound the regret of \algExploreExploit against that of \sfgpopt. It is easier to directly analyze different algorithms and then compare the regret bounds.}
% \end{proof}

%%% Local Variables:
%%% mode: latex
%%% TeX-master: "main"
%%% End:
