# Supplementary material for: A General Framework for Multi-fidelity Bayesian Optimization with Gaussian Processes
Source: arXiv:1811.00755 source file (2018-11-02)
Supplement: Supplementary file 2 [file appendix-proof-infogain.tex]

\section{Supplemental Results on Regret Analysis}
% \clearpage
% \section{Information gain of \algref{alg:explorelf}}

% \begin{theorem}[Greedy information gain]
% \end{theorem}

% \begin{corollary}[Cumulative regret with the information gain bound]
% \end{corollary}

Note that the regret bound in \thmref{thm:general:datadependent-bound} depends on $\gamma_\eplow$, which cannot be computed unless we run the algorithm. Ideally, we would like to obtain a bound prior to running the algorithm. In the following, we state a variant of the above bound, given some additional assumptions about $\beta_j$.  % and the joint distribution $\mathbb{P}$ over $\utility_1, \dots, \utility_\targetfid$. 
\begin{theorem}% [Data-independent bound on the cumulative regret]
  \label{thm:alg-independent-bound}
  % Let us set $\beta_1, \dots, \beta_k$ such that
  % Then, it holds that the average cumulative regret of \algname
  Assume $\beta_1\leq \dots \leq \beta_k$, and $\sum_j \beta_j^{-1} = \littleO{\sqrt{\budget}}$. We make further assume on the joint GP distribution, such that the mutual information between $\tarf$ and any set of actions is submodular\footnote{Note that this is trivial in the single-fidelity setting.}.
  Assume that \sfgpopt satisfy the same regret bound as in \thmref{thm:general:datadependent-bound}. Then, the cumulative regret of \algname satisfies
  \begin{align*}
    \cumreg(\policy,\budget) \leq \sqrt{\constgeneral_1 \budget \paren{\gamma - \gamma_1}} + \constgeneral_2\gamma_\eplow(\beta_1) \cdot \littleO{\sqrt{\budget}}
  \end{align*}
  with high probability, where $C_1, C_2$ are constants independent of $\budget$, $\gamma$ is the maximal information gain possible under budget $\budget$, $\gamma_1$ is the mutual information obtained by \explorelf (\algref{alg:explorelf}) in the first iteration of \algname (with no previous actions selected), and $\gamma_\eplow(\beta_1)$ is obtained by running \algref{alg:greedylf} with $\beta_1$.
\end{theorem}

Note that the above regret bound does not depend on the full $\gamma_\eplow$ as is the case for \thmref{thm:general:datadependent-bound} (i.e., it does not require us to run \algname till the end to compute the bound).
% To bound $\max_j \eplowcostat{j}$,
Before we provide the proof of \thmref{thm:alg-independent-bound}, we first establish the following lemma.
% Recall that the low fidelity cost at the $j^{\text{th}}$ episode satisfies
% \begin{align*}
%   \frac{\condinfgain{\bobs_{\eplow}^{(j)} }{\bobs_{\epselected}^{(1:j-1)}}}{\eplowcostat{j} } \geq \beta_j
% \end{align*}

\begin{lemma}\label{lm:ratio-monotone}
  Let $\mathcal{V} = \{v_1, \dots, v_n\}$. Each item $v_i \in \mathcal{V}$ is associated with a cost $c(\{v_i\})$, where $c(\selsubset) = \sum_{v\in \selsubset} c(\{v\})$ for $\selsubset \subseteq \mathcal{V}$ and $c(\emptyset) = 0$. Let $f:2^{\mathcal{V}} \rightarrow \NonNegativeReals$ be a monotone submodular utility function, and $g(\budget) := \max_{c(\selsubset) \leq \budget} f(\selsubset)$ be the maximal utility under budget $\budget\geq 0$. Then, $\forall \budget_2 \geq \budget_1 \geq 0$,
  \begin{align*}
    % \frac{\max_{c(S) \leq x+c_n}f(S)}{B} \geq \frac{\max_{c(S) \leq x'}f(S)}{x'}
    \frac{g(\budget_1+c_{\max})}{\budget_1} \geq \frac{g(\budget_2)}{\budget_2}
  \end{align*}
  where $c_{\max} = \max_{v\in \mathcal{V}} c(\{v\})$ is the maximal item cost.
\end{lemma}
\begin{proof}
  Fix $\budget_2 > 0$. Let $\maxset_2$ be a set which achieves the maximal utility under budget $\budget_2$, i.e., $\maxset_2 = \argmax_{c(\selsubset) \leq \budget_2}f(\selsubset)$, and $t=|\maxset_2|$.
  Assume that the items in $\maxset_2$ is sorted into a sequence $\paren{\maxsetat{1}_2, \maxsetat{2}_2, \dots, \maxsetat{t}_2}$, such that
  \begin{align}
    \frac{\utilgain{\maxsetat{1}_2 }{ \emptyset}}{c\paren{\maxsetat{1}_2}}
    \geq \frac{\utilgain{\maxsetat{2}_2}{\maxsetoflen{1}_2}}{c\paren{\maxsetat{2}_2}}
    \geq \dots
    \geq \frac{\utilgain{\maxsetat{t}_2}{\maxsetoflen{t-1}_2}}{c\paren{\maxsetat{t}_2}} \label{eq:app:sub:sorted}
  \end{align}
  % \begin{align*}
  %   \frac{f\paren{\maxsetat{1}_2}}{c\paren{\maxsetat{1}_2}}
  %   \geq \frac{f\paren{\maxsetoflen{2}_2} - f\paren{\maxsetat{1}_2}}{c\paren{\maxsetat{2}_2}}
  %   \geq \dots
  %   \geq \frac{f\paren{\maxsetoflen{t}_2} - f\paren{\maxsetoflen{t-1}_2}}{c\paren{\maxsetat{2}_2}}
  % \end{align*}
  where $\maxsetoflen{\tau}_2 = (\maxsetat{1}_2, \dots \maxsetat{\tau}_2)$ denotes the (sorted) sequence of length $\tau$, and $\utilgain{v}{\selsubset} := f\paren{\selsubset \cup \{v\}} - f\paren{\selsubset}$.

  Now, for any $\budget_1 \in (0, \budget_2)$, let $t_1$ be the index of the item in $\maxsetoflen{t}_2$ such that
  \begin{align}
    c\paren{\maxsetoflen{t_1 - 1}} \leq \budget_1 \leq c\paren{\maxsetoflen{t_1}}. \label{eq:app:sub:cost:lb}
  \end{align}
  We know
  \begin{align}
    c\paren{\maxsetoflen{t_1}}
    &= c\paren{\maxsetoflen{t_1 - 1}} + c\paren{\maxsetat{t_1}}\nonumber \\
    &\stackrel{}{\leq} c\paren{\maxsetoflen{t_1 - 1}} + \max_{v\in \mathcal{V}} c(\{v\})\nonumber \\
    &\stackrel{\eqref{eq:app:sub:cost:lb}}{\leq} \budget_1 + \max_{v\in \mathcal{V}} c(\{v\}) \nonumber \\
    &= \budget_1 + c_{\max}. \label{eq:app:sub:cost:ub}
  \end{align}
  By the monotonicity of $f$,
  \begin{align}
    f\paren{\maxsetoflen{t_1}}
    \leq \max_{c\paren{\selsubset} \leq c\paren{\maxsetoflen{t_1}}} f\paren{\selsubset}
    \stackrel{\eqref{eq:app:sub:cost:ub}}{\leq} \max_{c\paren{\selsubset} \leq \budget_1 + c_{\max}} f\paren{\selsubset}. \label{eq:app:sub:util:ub}
  \end{align}
  Combining Eq.~\eqref{eq:app:sub:cost:lb} and \eqref{eq:app:sub:util:ub} we get
  \begin{align}
    \label{eq:app:sub:utilcostratio:temp1}
    \frac{f\paren{\maxsetoflen{t_1}}}{c\paren{\maxsetoflen{t_1}}} \leq \frac{\max_{c\paren{\selsubset} \leq \budget_1 + c_{\max}} f\paren{\selsubset}}{\budget_1} = \frac{g(\budget_1+c_{\max})}{\budget_1}.
  \end{align}
  Further, from Eq.~\eqref{eq:app:sub:sorted} we obtain
  \begin{align*}
    \frac{f\paren{\maxsetoflen{t_1}}}{c\paren{\maxsetoflen{t_1}}}
    \stackrel{(a)}{\geq} \frac{\utilgain{\maxsetat{t_1+1}_2}{\maxsetoflen{t_1}_2}}{c\paren{\maxsetat{t_1+1}_2}}
    \geq \dots
    \geq \frac{\utilgain{\maxsetat{t}_2}{\maxsetoflen{t-1}_2}}{c\paren{\maxsetat{t}_2}}
  \end{align*}
  where step (a) is by the fact that $\frac{a_1}{b_1} \geq \frac{a_2}{b_2} \Rightarrow \frac{a_1}{b_1} \geq \frac{a_1+a_2}{b_1+b_2} \geq \frac{a_2}{b_2}$ for $b_1,b_2> 0$. Apply this inequality once again, we get
  \begin{align}
    \frac{f\paren{\maxsetoflen{t_1}}}{c\paren{\maxsetoflen{t_1}}}
    \geq \frac{f\paren{\maxsetoflen{t}}}{c\paren{\maxsetoflen{t}}}
    = \frac{g(\budget_2)}{\budget_2} \label{eq:app:sub:utilcostratio:temp2}.
  \end{align}
  Combining Eq.~\eqref{eq:app:sub:utilcostratio:temp1} with \eqref{eq:app:sub:utilcostratio:temp2} hence completes the proof.
\end{proof}

\begin{algorithm}[h]
  \nl {\bf Input}: $\mathcal{V}$; budget $\budget$; cost $c\paren{\epselected}$ for $\selsubset \subseteq \mathcal{V}$; utility function $f$ \\ % between $\fidelity_i$ and noise $$. \\
  \Begin{
    \nl $\epselected_1 \leftarrow
    \argmax \curlybracket{f\paren{v}: c\paren{\{v\}} \leq \budget}$ \tcc*{best single element solution}
    \nl $\epselected_2 \leftarrow \emptyset$ \\
    % \nl $\Cost_\epselected \leftarrow 0$  \\ % \tcc*{cost of selected items}
    \While{$c\paren{\epselected_2} \leq \budget$}
    {
      \nl $v^* \leftarrow
      \argmax_{v} \curlybracket{\frac{f\paren{\epselected_2 \cup \{v\}} - f\paren{\epselected_2}}{c\paren{v}}: c\paren{\epselected_2 \cup \{v\}} \leq \budget}$       \tcc*{greedy benefit-cost ratio, low-fidelities}
      \If{ $v^* =\nan$}
      {
        \nl break \tcc*{exceeding budget, stop}
      }
      \Else
      {
        \nl $\epselected_2 \leftarrow \epselected_2 \cup \{v^*\}$
      }
    }
    \nl {\bf Output}: $\argmax_{\epselected \in \{\epselected_1, \epselected_2\}}f(\epselected)$ \\
  }
  \caption{Submodular maximization under knapsack constraints (Algorithm 1 of \citet{krause2005note}).}\label{alg:greedyks} % \algGreedyLF
\end{algorithm}

\begin{lemma}[Adapted from \citet{krause2005note}]\label{lm:greedyks}
  Let $\mathcal{V} = \{v_1, \dots, v_n\}$. Each item $v_i \in \mathcal{V}$ is associated with a cost $c(\{v_i\})$, where $c(\selsubset) = \sum_{v\in \selsubset} c(\{v\})$ for $\selsubset \subseteq \mathcal{V}$. Let $f:2^{\mathcal{V}} \rightarrow \NonNegativeReals$ be a monotone submodular utility function, and $\epselected$ be the solution returned by \algref{alg:greedyks} under budget $\budget \geq 0$. Then,
  \begin{align*}
    f(\epselected) \geq \frac12\paren{1-\frac{1}{e}} g(\budget)
  \end{align*}
  where $g(\budget) := \max_{c(\selsubset) \leq \budget} f(\selsubset)$ is the maximal utility under budget $\budget$.
\end{lemma}

We then establish the following lemma.
\begin{algorithm}[h]
  \nl {\bf Input}: $\beta$; total budget $\budget$, joint GP prior on $\{\fidelity_i, \noise_i\}_{i\in[\targetfid]}$\\ % between $\fidelity_i$ and noise $$. \\
  \Begin{
    \nl $\gamma_{\max} \leftarrow 0$ \\
    \nl $c_{\max} \leftarrow \max\curlybracket{\costof{\fid}: \fid\neq \targetfid}$ \\ % \tcc*{selected items}

    \nl $\epselected_1 \leftarrow
    \argmax_{\action{\ex, \fid}} \curlybracket{\infgain{\obs_{\action{\ex, \fid}}}: \fid \neq \targetfid}$ \tcc*{low fidelity action with the largest information gain}
    \nl $\epselected_2 \leftarrow \emptyset$ \\
    % \nl $\Cost_\epselected \leftarrow 0$  \\ % \tcc*{cost of selected items}
    \While{$c\paren{\epselected_2} \leq \budget$}
    {
      \nl $\action{\ex^*, \fid^*} \leftarrow
      \argmax_{\action{\ex, \fid}} \curlybracket{\frac{\condinfgain{\obs_{\action{\ex, \fid}}}{\bobs_{\epselected}}}{\costof{\fid}}: \fid \neq \targetfid}$       \tcc*{greedy benefit-cost ratio, low-fidelities}
      \nl $\epselected_2 \leftarrow \epselected_2 \cup \{\action{\ex^*,\fid^*}\}$ \\
      \nl $\gamma_{\max} \leftarrow \frac{\max\curlybracket{\infgain{\bobs_{\epselected_1}}, \infgain{\bobs_{\epselected_2}}}}{\frac{1}{2}\paren{1-\frac{1}{e}}}$ \tcc*{pick the better solution between $\epselected_1$ and $\epselected_2$} \label{ln:alg:greedylf:scaledgreedy}
      % \nl $\gamma_{\max} \leftarrow \frac{\gamma_{\max}}{\frac{1}{2}\paren{1-\frac{1}{e}}}$ \\
      \If{ $c\paren{\epselected_2} \leq c_{\max}$} {\nl continue \tcc*{keep growing $\epselected_2$}}
      % \If{$\frac{\gamma_{\max}}{c\paren{\epselected_2} - c_{\max}} < \frac{\beta}{2}\paren{1-\frac{1}{e}}$}
      \If{$\frac{\gamma_{\max}}{c\paren{\epselected_2} - c_{\max}} < \beta$}
      % \If{ $\fid^* = \nan$ or $\frac{\condinfgain{\bobs_{\epselected \cup \{ \action{\ex^*, \fid^*} \} } }{\bobs_\selected}} {\paren{\Cost_\epselected + \costof{\fid^*}}} < \beta \frac{1-e}{2e}$}
      {
        \nl break \tcc*{if $\beta\leq \min_{j}{\beta_j}$, \label{ln:alg:greedylf:stopping}% then by \lemref{lm:ratio-monotone},
          $\gamma_{\max}$ is an upper bound of the information gain of \algref{alg:explorelf}} \label{alg:greedygain:ln:infgaincheck}
      }
    }
    \nl {\bf Output}: $\gamma_{\max}$ \\
  }
  \caption{Greedy algorithm for computing the upper bound on $\gamma_{\max}$}\label{alg:greedylf} % \algGreedyLF
\end{algorithm}
\begin{lemma}\label{lem:gammamax}
  Let $\gamma_{\max}$ be the output for \algref{alg:greedylf}. Then
  \begin{align*}
    \gamma_{\max} \geq \max_{j} \condinfgain{\bobs_{\eplow}^{(j)} }{\bobs_{\epselected}^{(1:j-1)}}
  \end{align*}
\end{lemma}
\begin{proof}
%   By the fact that the conditional joint distribution of $\bobs_{\eplow}^{(j)}$ and $\tarf$ is a joint Gaussian (process) distribution, we know that the mutual information function is non-negative and monotone submodular. % \yuxin{True??} % (note that different from the mutual information between )
  By the assumption of \thmref{thm:alg-independent-bound}, and the fact that the conditional joint distribution of $\bobs_{\eplow}^{(j)}$ and $\tarf$ is a joint Gaussian (process) distribution, we know that the mutual information function is non-negative and monotone submodular. 
  From \lemref{lm:greedyks} we know that the scaled greedy solution $\gamma_{\max}$ at \lnref{ln:alg:greedylf:scaledgreedy} of \algref{alg:greedylf} is an upper bound on the maxial information gain under budget $c(\epselected_2)$. Combining the stopping condition at \lnref{ln:alg:greedylf:stopping} of \algref{alg:greedylf} with \lemref{lm:ratio-monotone} completes the proof.
\end{proof}

Now we are ready to prove \thmref{thm:alg-independent-bound}.
\begin{proof}[Proof of \thmref{thm:alg-independent-bound}]
  % Assume $\beta_1\leq \dots \leq \beta_k$, and $\sum_j \beta_j^{-1} = \littleO{\sqrt{\budget}}$.
  % Assume $\sum_j \beta_j^{-1} = \littleO{\sqrt{\budget}}$.
  We first bound the first term of the RHS of Eq.~\eqref{eq:general-regret-intermediate}. From Eq.~\eqref{eq:app:sumeplowcostbound} we know
  \begin{align}
    \sum_{j=1}^k{\eplowcostat{j}}
    &\leq \sum_{j=1}^k\frac{\condinfgain{\bobs_{\eplow}^{(j)} }{\bobs_{\epselected}^{(1:j-1)}}}{\beta_j}
      \nonumber \\
      % &\stackrel{}{\leq} \sum_{j=1}^k\frac{\max_{j}\condinfgain{\bobs_{\eplow}^{(j)} }{\bobs_{\epselected}^{(1:j-1)}}}{\beta_j} \nonumber \\
    &\stackrel{(a)}{\leq} \max_{j}\condinfgain{\bobs_{\eplow}^{(j)} }{\bobs_{\epselected}^{(1:j-1)}} \cdot \sum_{j=1}^k\beta_j^{-1} \nonumber \\
    &\stackrel{}{=} \underbrace{\max_{j}\condinfgain{\bobs_{\eplow}^{(j)} }{\bobs_{\epselected}^{(1:j-1)}}}_{\leq \gamma_\eplow(\beta_1)} \cdot \ \littleO{\sqrt{\budget}} \nonumber\\
    &\stackrel{\lemref{lem:gammamax}}{\leq} \gamma_\eplow(\beta_1) \cdot \ \littleO{\sqrt{\budget}}
  \end{align}
  where step (a) is by the assumption $\sum_j \beta_j^{-1} = \littleO{\sqrt{\budget}}$. Therefore,
  \begin{align*}
    \frac{\tarf^*}{\costof{\targetfid}} \cdot \sum_{j=1}^k{\eplowcostat{j}}  \leq \frac{\tarf^*}{\costof{\targetfid}} \cdot \gamma_\eplow(\beta_1) \cdot \ \littleO{\sqrt{\budget}}
  \end{align*}
  % As annotated in the above equation, let $\gamma_\eplow^{\max} = \max_{j}\condinfgain{\bobs_{\eplow}^{(j)} }{\bobs_{\epselected}^{(1:j-1)}}$ be the maximum information gain of the lower fidelities of any episode. % by $\gamma_\eplow^{\max}$ as annotated above
  % To bound the regret from exploring the low fidelity actions, it suffices to find an upper bound on $\gamma_\eplow^{\max}$.

  % Let $\eplow' = \{\action{\ex_\tau, \fid_\tau}\}_{\tau\in[t]}$ be any set of low fidelity actions (i.e., $\fid_\tau \neq \targetfid$), and $\bobs_{\eplow'} = \{\utility_{\fid_\tau}(\ex)\}_{\tau\in[t]}$, $ \Cost_{\eplow'} = \sum_{\tau\in[t]} \costof{\fid_\tau}$ be the observations and total cost of the actions in $\eplow'$, respectively.  Then $\forall j \in [k]$,
  % \begin{align*}
  %   \condinfgain{\bobs_{\eplow}^{(j)} }{\bobs_{\epselected}^{(1:j-1)}}
  %   \stackrel{(a)}{\leq} \infgain{\bobs_{\eplow}^{(j)} }
  %   \stackrel{}{\leq} \max_{\Cost_{\eplow'} \leq \eplowcostat{j}}\infgain{\bobs_{\eplow'}}
  % \end{align*}
  % where step (a) is by submodularity of mutual information. Taking the maximum over $j$ from both sides,
  % \begin{align}
  %   \gamma_\eplow^{\max}
  %   = \max_j \condinfgain{\bobs_{\eplow}^{(j)} }{\bobs_{\epselected}^{(1:j-1)}}
  %   %   &\leq \max_j \infgain{\bobs_{\eplow}^{(j)} } \\
  %   \leq \max_j \max_{\eplow': \Cost_{\eplow'} \leq \eplowcostat{j}}\infgain{\bobs_{\eplow'}}
  %   = \max_{\Cost_{\eplow'} \leq \max_j \eplowcostat{j}}\infgain{\bobs_{\eplow'}}
  % \end{align}
  %     % \begin{lemma}[Bounds on $\gamma_m$, $\gamma_\eplow$] \yuxin{TBD}
  %     % \end{lemma}
  %     % \begin{proof}
  Now let us focus on the second term of Eq.~\eqref{eq:general-regret-intermediate}. It is the regret of \sfgpopt on the target fidelity, under budget $\budget-\sum_{j=1}^k{\eplowcostat{j}}$. By the assumption on the regret of \sfgpopt,
  \begin{align*}
    \sum_{j=1}^{k} \paren{\tarf^* - \tarf(\ex_j)}
    &\leq \sqrt{C \paren{\budget-\sum_{j=1}^k{\eplowcostat{j}}} \sum_{j=1}^k {\condinfgain{\obs_{\targetfid}^{(j)} }{\bobs_{\epselected}^{(1:j-1)} \cup \bobs_{\eplow}^{(j)}}}}\\
    &\leq \sqrt{C \budget \sum_{j=1}^k {\condinfgain{\obs_{\targetfid}^{(j)} }{\bobs_{\epselected}^{(1:j-1)} \cup \bobs_{\eplow}^{(j)}}}}
  \end{align*}

  By the chain rule of mutual information, we know
  \begin{align*}
    \condinfgain{\bobs_{\epselected}^{(j)}}{\bobs_{\epselected}^{(1:j-1)}}
    &= \condinfgain{\bobs_{\eplow}^{(j)}, \obs_{\targetfid}^{(j)}}{\bobs_{\epselected}^{(1:j-1)}} \\
    &= \condinfgain{\obs_{\targetfid}^{(j)} }{\bobs_{\epselected}^{(1:j-1)}, \bobs_{\eplow}^{(j)}} + \condinfgain{\bobs_{\eplow}^{(j)} }{\bobs_{\epselected}^{(1:j-1)}}.
  \end{align*}
  Therefore
  \begin{align}
    \sum_{j=1}^k\condinfgain{\obs_{\targetfid}^{(j)} }{\bobs_{\epselected}^{(1:j-1)}, \bobs_{\eplow}^{(j)}}
    &= \infgain{\bobs_{\epselected}^{(1:k)} }- \sum_{j=1}^k\condinfgain{\bobs_{\eplow}^{(j)} }{\bobs_{\epselected}^{(1:j-1)}}  \nonumber \\
    &\leq \max_{\selected: \costOfSet{\selected} \leq \budget}\infgain{\bobs_{\selected}} - \sum_{j=1}^k\condinfgain{\bobs_{\eplow}^{(j)} }{\bobs_{\epselected}^{(1:j-1)}}\nonumber \\
    &= \max_{\selected: \costOfSet{\selected} \leq \budget}\infgain{\bobs_{\selected}} - \gamma_\eplow\nonumber
    % \max_{\selectedTar: \costOfSet{\selectedTar}\leq \budget - \epcost}\condinfgain{\bobs_{\selectedTar}}{\bobs_\eplow}
    % &\leq \max_{\selected: \costOfSet{\selected} \leq \budget}\infgain{\bobs_{\selected}} - \infgain{\bobs_{\eplow}} = \gamma - \gamma_\eplow.
  \end{align}
  Let $\gamma_m = \max_{\selected: \costOfSet{\selected} \leq \budget}\infgain{\bobs_{\selected}}$ be the mutual information gathered can be gathered under budget $\budget$, We thus have
  \begin{align}
    \sum_{j=1}^{k} \paren{\tarf^* - \tarf(\ex_j)} &\leq \sqrt{C \paren{\budget-\epcost} (\gamma - \gamma_\eplow)} \leq \sqrt{C \budget (\gamma - \gamma_\eplow)} \leq \sqrt{C \budget (\gamma - \gamma_1)}. \label{eq:targetfid_infgain_ub}
  \end{align}
  Combining Eq.~\eqref{eq:general-cost-lf-ub}, \eqref{eq:targetfid_infgain_ub} with Eq.~\eqref{eq:general-regret-intermediate} completes the proof.
  % \end{proof}
\end{proof}

%%% Local Variables:
%%% mode: latex
%%% TeX-master: "main"
%%% End:
