# Supplementary material for: A General Framework for Multi-fidelity Bayesian Optimization with Gaussian Processes
Source: arXiv:1811.00755 source file (2018-11-02)
Supplement: Supplementary file 3 [file appendix-exp.tex]

\section{Supplemental Experimental Results}

%%% Local Variables:
%%% mode: latex
%%% TeX-master: "main"
%%% End:
